# Supplementary material for: Segment Any 3D Object with Language
Source: arXiv:2404.02157 source file (2024-04-02)
Supplement: Supplementary file 1 [file trashcan.pdf]

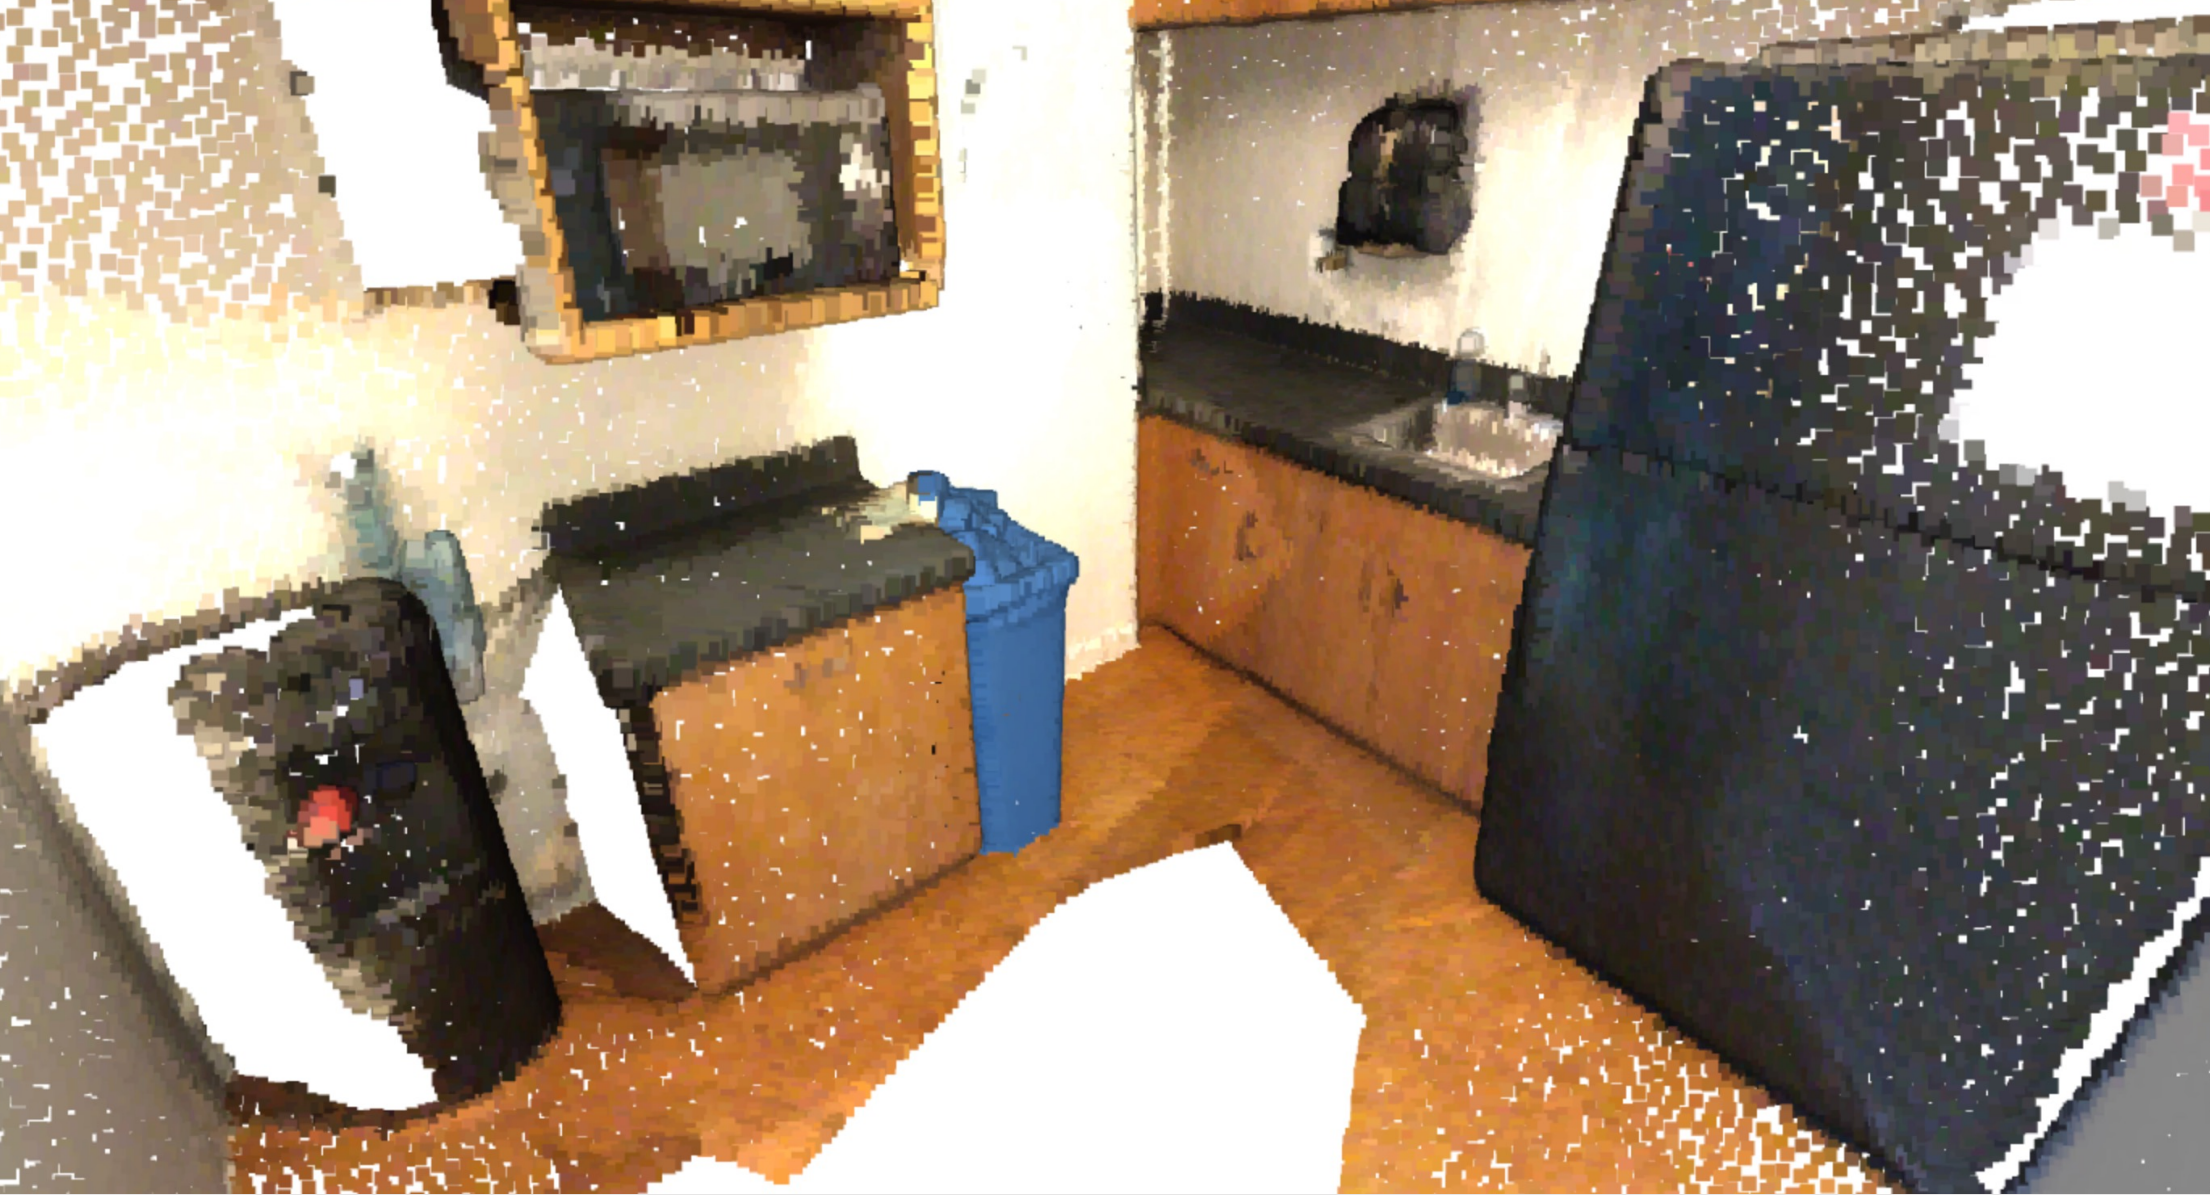

a **trash can** with a microwave on top of it



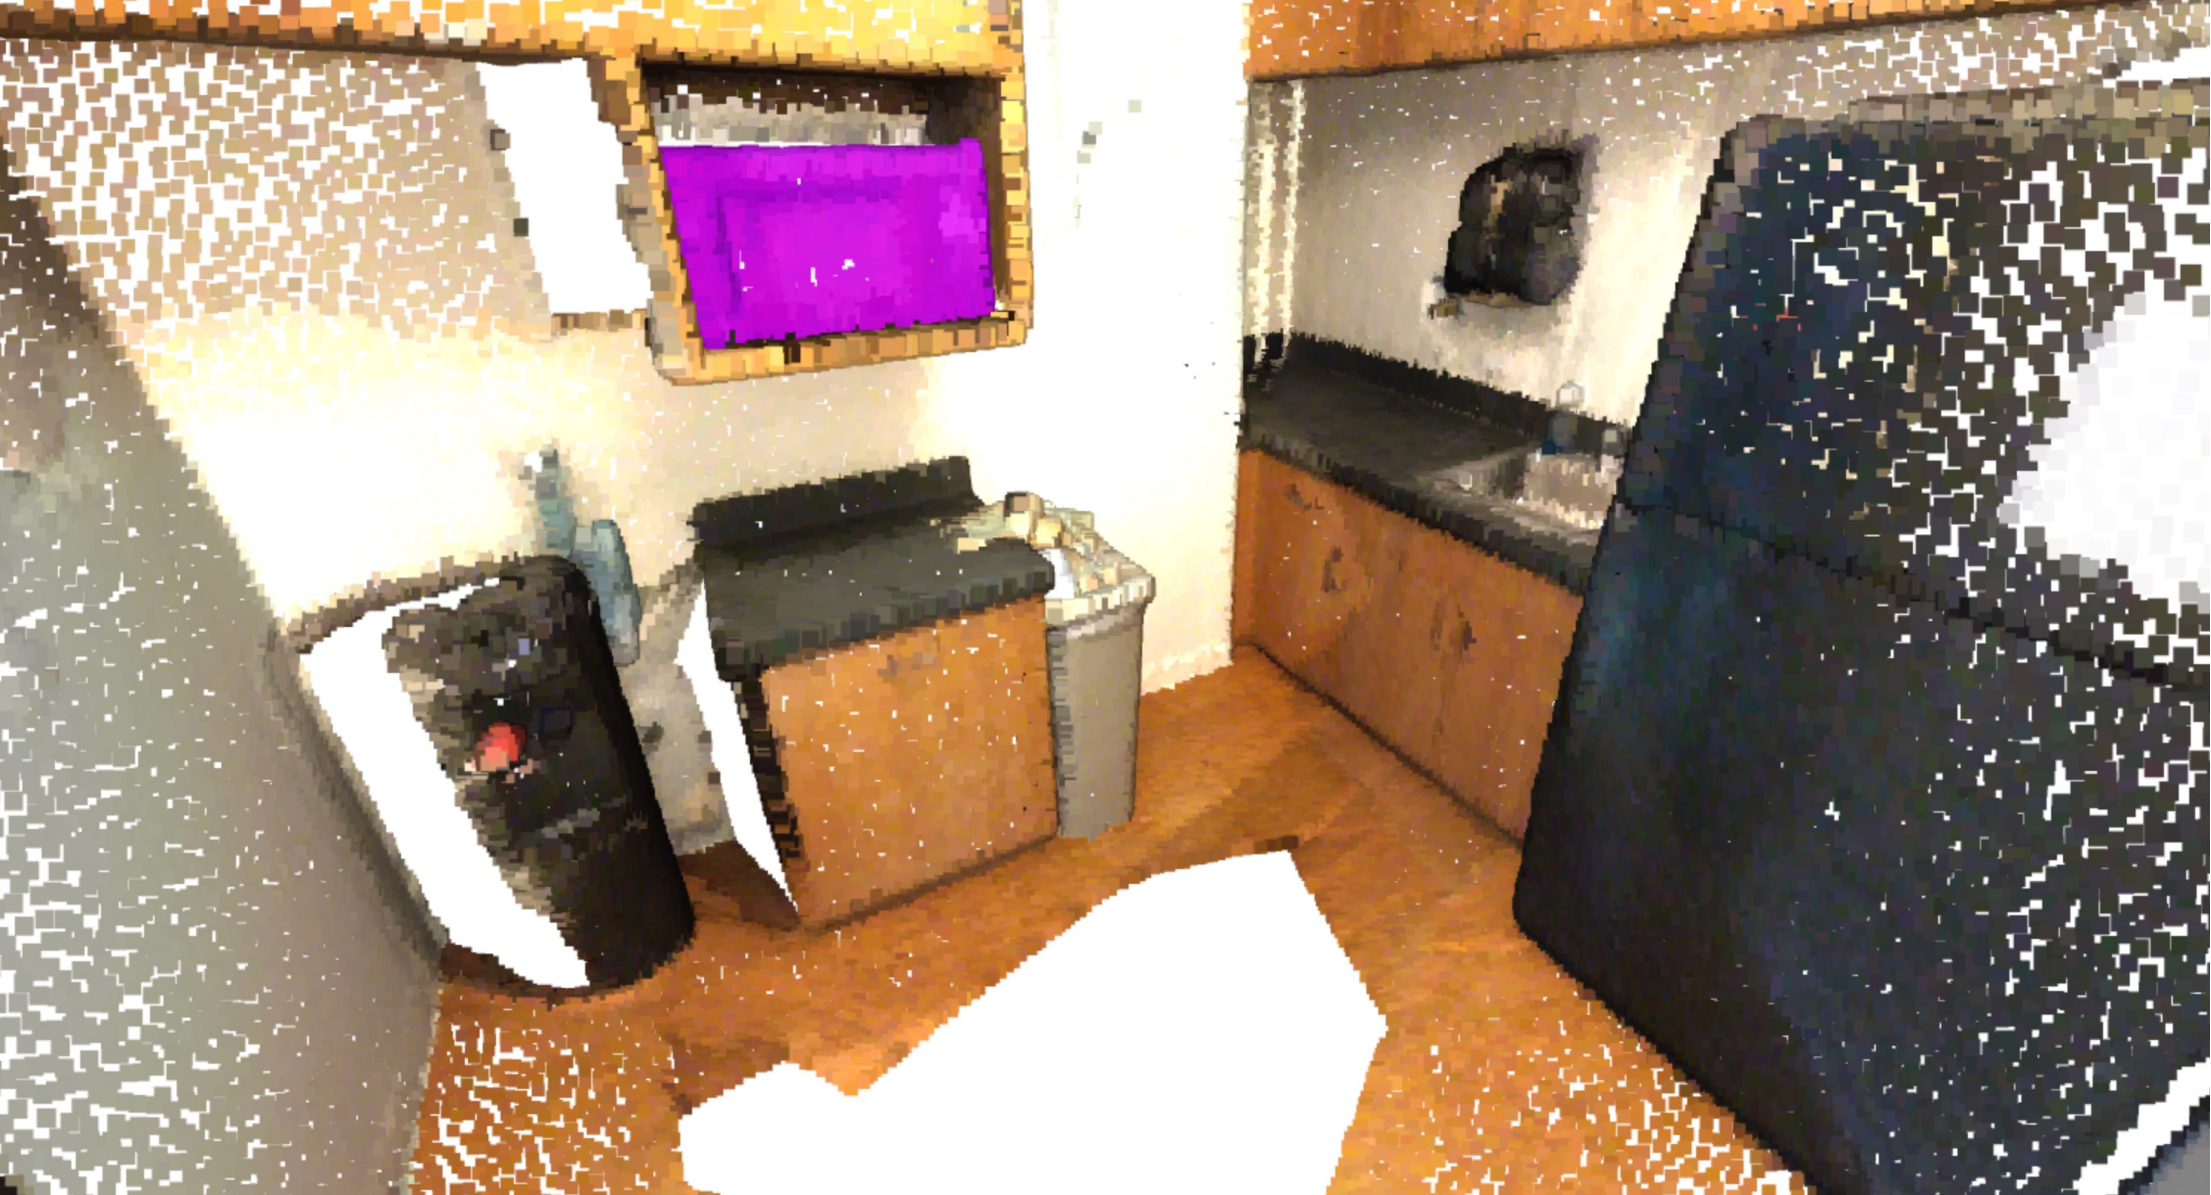

a microwave oven sitting inside of a small kitchen
